# Supplementary material for: BEVFormer v2: Adapting Modern Image Backbones to Bird's-Eye-View Recognition via Perspective Supervision
Source: arXiv:2211.10439 source file (2022-11-18)
Supplement: Supplementary file 1 [file appendix_depth_pretrained.tex]

\setlength{\tabcolsep}{3pt}
\setlength{\doublerulesep}{2\arrayrulewidth}

\begin{table*}[t]
    \caption{3D detection results on the nuScenes \emph{test} set of BEVFormer v2 with a COCO pre-trained VoVNet-99 and a depth pre-trained VoVNet-99. We omit the pre-training epochs for COCO since COCO pre-trained backbones are widely available and both settings use the same COCO pre-training. }
    \label{table:depth_pretrain}
    \centering

    \begin{tabular}{c|c|c|cc|cccccc}
        \toprule
        Backbone & Epoch & Pre-train & NDS & mAP & mATE & mASE & mAOE & mAVE & mAAE   \\ 
        \midrule
        DLA-34 & 72 & COCO & & & & & & & & \\ 
        DLA-34 & \small{15M Img + 120 + 24} & \small{COCO $\xrightarrow{}$ DDAD15M $\xrightarrow{}$ nuScenes} & & & & & & & \\ 
        \midrule
        VoVNet-99 & 72 & COCO & & & & & & & & \\ 
        VoVNet-99 & \small{15M Img + 120 + 24} & \small{COCO $\xrightarrow{}$ DDAD15M $\xrightarrow{}$ nuScenes} & & & & & & & \\ 
        \bottomrule
    \end{tabular}
\end{table*}
