# Supplementary material for: BEVFormer v2: Adapting Modern Image Backbones to Bird's-Eye-View Recognition via Perspective Supervision
Source: arXiv:2211.10439 source file (2022-11-18)
Supplement: Supplementary file 2 [file appendix_long_schedule.tex]

\setlength{\tabcolsep}{3pt}
\setlength{\doublerulesep}{2\arrayrulewidth}

\begin{table*}[ht]
    \caption{3D detection results on the nuScenes \emph{test} set with a extended training schedule for InterImage-XL.}
    \label{table:extend_training}
    \centering

    \begin{tabular}{c|c|cc|cccccc}
        \toprule
        Backbone & Epoch & NDS & mAP & mATE & mASE & mAOE & mAVE & mAAE   \\ 
        \midrule
        InternImage-XL & 24 & & & & & & & \\ 
        InternImage-XL & 48 & & & & & & & \\ 
        InternImage-XL & 72 & & & & & & & \\ 
        \bottomrule
    \end{tabular}
    
\end{table*}
